# Supplementary material for: Fast Robust Subspace Tracking via PCA in Sparse Data-Dependent Noise
Source: arXiv:2006.08030 source file (2020-12-04)
Supplement: Supplementary file 1 [file appendix_possibly_delete.tex]

%
%
%Let $\Phat_{j,0} = \Phat_{(t)}$ denote the estimated subspace from the interval. We will show that $\SE(\Phat_{j,0},\P_j) \le 2.5 (3 \Delta + 0.36 (\zz + \Delta) + \zz^2) \le 10 \Delta$.
%Define $(\e_{\l})_t = \bm{I}_{\Tt}\left(\bpsi_{\Tt}{}'\bpsi_{\Tt}\right)^{-1} \I_{\Tt}{}' \bpsi \lt$ and $(\e_{\v})_t = \bm{I}_{\Tt}\left(\bpsi_{\Tt}{}'\bpsi_{\Tt}\right)^{-1} \I_{\Tt}{}' \bpsi \vt$.
%
%Apply the result with

\section{Proof of PCA-SDDN Corollary with Subspace Change and Most General PCA Result} \label{sec:pca_app}

\subsection{Proof of Corollary \ref{pca_ssch}} \label{proof_pca_ssch}
\begin{proof}[Proof of Corollary \ref{pca_ssch}]
We again apply the sin theta theorem,  Lemma \ref{sintheta}, with $\bm{D} = \frac{1}{\tmaxpca}\sum_t \yt \yt{}'$.  $\Phat$ is the matrix of top $r$ eigenvectors of $\bm{D}$.  But we need to pick $\D_0$ more carefully now. Let
\[
\D_0 = \frac{1}{\alpha}  \P \left(  (\alpha-\alpha_0) \Lam +  \alpha_0 \P' \P_0  \Lam \P_0' \P \right) \P'
\]
This is a Hermitian matrix as needed by the sin theta theorem, and $\P$ is its matrix of top $r$ eigenvectors. Moreover, it is rank $r$, so that $\lambda_{r+1}(\D_0) = 0$.
%By Lemma \ref{sintheta},
%\[
%\SE(\Phat,\P) \leq  \frac{\| \D - \D_0\|}{\lambda_{r}(\D_0) - \lambda_{r+1}(\D_0) - \| \D - \D_0\|}
%\]
Notice that
\begin{align*}
\D - \D_0 &= \cross + \cross{}' +  \noise  \\
&+ \left(\frac{1}{\alpha} \sum_t \lt \lt'  - \E[\frac{1}{\alpha} \sum_t \lt \lt'] \right) +  \left( \E[\frac{1}{\alpha} \sum_t \lt \lt'] - \D_0 \right)
%
%\frac{1}{\tmaxpca} \sum_t \yt \yt{}' - \D_0 = ??
%\frac{1}{\tmaxpca} \sum_t \lt \wt{}' + \wt \lt{}'  + \wt \wt{}' + \bv \bv{}' + \bv \wt{}' + \wt \bv{}' + \lt \bv{}' + \bv \lt{}'  \\
%&:= \cross_{\l, \w} + \cross_{\l, \w}{}' + \noise_{\w} + \noise_{\bv} + \cross_{\l, \bv} + \cross_{\l, \bv}{}' + \cross_{\bv,\w} + \cross_{\bv,\w}{}' \\
%&= \cross + \cross{}' +  \noise
\end{align*}
where $\cross, \noise$ are as defined earlier with the change that $\lt$ is now defined differently. {\em Thus, the only thing that changes when bounding these is our definition of $q$. We now let $q$ be the upper bound on
$\max(\|\Mtone \P_0\|, \|\Mtone \P\|)$.}

For our current model, we have $\sum_t \lt \lt' = \alpha_0 \P_0 \Lam \P_0' + (\alpha - \alpha_0) \P \Lam \P'$.
Since we can always express $\P_0 $ as $\P_0 = \P \P' \P_0 + \P_\perp \P_\perp{}' \P_0$, we have
\begin{align*}
&\frac{1}{\alpha} \E[\sum_t \lt \lt' ] \\
& = \D_0 + c_0 \P_\perp \P_\perp' \P_0  \Lam \P_0' \P_\perp \P_\perp{}'  + c_0 \P_\perp \P_\perp' \P_0  \Lam \P_0' \P \P' + (.)'
\end{align*}
with $c_0: = \frac{\alpha_0}{\alpha}$.

From our assumption, $\|\P_\perp \P_\perp' \P_0\| \le \Delta$, $\|\P' \P_0\| \le 1$ and $\sigma_{\min}(\P' \P_0) \ge \sqrt{1-\Delta^2}$. Thus,
\[
 \| \E\left[\frac{1}{\alpha} \sum_t \lt \lt'\right] - \D_0 \| \le c_0 \|\P_\perp' \P_0\|^2 \lambda^+ + 2 c_0 \|\P_\perp' \P_0\| \lambda^+  \le 3 c_0 \Delta  \lambda^+
\]
and
\begin{align*}
&\lambda_{r}(\D_0) \\
 & = \frac{1}{\alpha} \lambda_{\min}(  ( (\alpha-\alpha_0) \Lam + (\alpha_0) \P' \P_0  \Lam \P_0' \P ) )  \\
& \ge (1-c_0) \lambda^- + c_0 \sigma_{\min}^2(\P' \P_0) \lambda^- \ge (1-c_0) \lambda^- + c_0 (1-\Delta^2) \lambda^- = (1 - c_0 \Delta^2) \lambda^-
\end{align*}

Thus, applying  Lemma \ref{sintheta}, and using $\lambda_{r+1}(\D_0) = 0$,
\begin{align*}
&\SE(\Phat,\P)  \leq  \frac{\| \D - \D_0\|}{\lambda_{r}(\D_0) - \lambda_{r+1}(\D_0) - \| \D - \D_0\|} \\
%& \leq \frac{\| \left(\frac{1}{\alpha} \sum_t \lt \lt'  - \E[\frac{1}{\alpha} \sum_t \lt \lt'] \right)\| + 3 c_0 \Delta  \lambda^+ + 2\|\cross\| + \|\noise\|}{\lambda_{r}(\D_0) - \mathrm{numerator}} \\
& \leq \frac{\| \left(\frac{1}{\alpha} \sum_t \lt \lt'  - \E\left[\frac{1}{\alpha} \sum_t \lt \lt'\right] \right)\| + 3 c_0 \Delta  \lambda^+ + 2\|\cross\| + \|\noise\|}{(1 - c_0 \Delta^2) \lambda^- - \mathrm{numerator}}
\end{align*}

To bound $\|\left(\frac{1}{\alpha} \sum_t \lt \lt'  - \E\left[\frac{1}{\alpha} \sum_t \lt \lt'\right] \right)\|$, we apply matrix Bernstein, see Theorem \ref{thm:matrix_bern}, with $\Z_t = \lt \lt'$. We have
\begin{align*}
\|\Z_t\| &\le \max(\|\P_0 \at \at' \P_0\|,\|\P \at \at' \P\|) = \|\at \at'\| \\
&= \|\at\|^2 \le \mu r \lambda^+ = R.
\end{align*}
Also, $\Z_t ' \Z_t = \Z_t \Z_t'$ and
\begin{align*}
&\|\sum_t \E[\Z_t \Z_t' ]\| \\
& = \|\sum_{t=1}^{\alpha_0} \P_0 \E[ \at \at' \P_0' \P_0 \at \at'] \P_0' +   \sum_{t= \alpha_0+1}^\alpha  \P \E[ \at \at' \P' \P \at \at'] \P'\| \\
& \le \max_t\|\at\|^2 \| \sum_{t=1}^{\alpha_0} \P_0 \Lam  \P_0 +   \sum_{t= \alpha_0+1}^\alpha  \P \Lam \P' \| \\
&\le R (\alpha_0 \lambda^+ + (\alpha-\alpha_0)\lambda^+)  = R \alpha \lambda^+
\end{align*}
Thus,
\[
\max( \|\frac{1}{\alpha} \sum_t \Z_t \Z_t' \|, \|\frac{1}{\alpha} \sum_t \Z_t{}' \Z_t \|) \le R \lambda^+  = \sigma^2
\]
By matrix Bernstein with $\epsilon  \equiv \epsilon \lambda^-$,  since $\alpha \ge \frac{1}{\epsilon^2} C f^2 \mu . r \log n$, w.p. at least $1 - 2 n^{-10}$,
\[
 \|\left(\frac{1}{\alpha} \sum_t \lt \lt'  - \E\left[\frac{1}{\alpha} \sum_t \lt \lt'\right] \right)\| \le \epsilon \lambda^-
\]
Thus,
\begin{align*}
\SE(\Phat,\P) & \leq \frac{3 c_0 \Delta  \lambda^+ + \epsilon \lambda^-  + 2\|\cross\| + \|\noise\|}{(1 - c_0 \Delta^2) \lambda^- - \mathrm{numerator}} \\
& \leq \frac{3 c_0 \Delta  \lambda^+ + \epsilon \lambda^-  + 4 \sqrt{\bz}q \lambda^+ + \lambda_v^+ + \epsbnd\lambda^-}{(1 - c_0 \Delta^2) \lambda^- - \mathrm{numerator}}
\end{align*}
The last bound follows using the bounds on $\cross, \noise$ from earlier.

Thus, if $4 c_0 \Delta f < 0.2$ and the bounds from the earlier result hold, then the denominator can be shown to  be greater than $0.4$. This finishes our proof.
\end{proof}

\subsection{Most General PCA Result}
Here we state our most general result for PCA in data-dependent noise.

\begin{definition}
Let
\ben
\item Let $\Lam_t = \E[\at \at{}']$, $\Lamb = \frac{1}{\tmaxpca}\sum_t \Lam_t$, $\lambda_{\max}^+ := \max_t \|\Lam_t\|$, $\lambda^-_{\avg} = \lambda_{\min}(\Lamb)$ and let $f = \lambda_{\max}^+/\lambda^-_{\avg}$ denote the ``effective condition number'' of $\Lamb$.
\item Define the following functions of $\bm\Sigma_{v,t}$:
\begin{align*}
&\lambda_{v,\P,\avg}^-:= \lambda_{\min}(\P'\bm\Sigvb \P),\\ 
&\Sig_{v,t,\rest} := \Sig_{v,t} - \P\P{}'\Sig_{v,t}\P\P{}',\\   
& \lambda_{v,\rest,\max}^+:= \max_t \lambda_{\max}(\Sig_{v,t,\rest}),
\end{align*}
and
\[
\lambda_{v,\P,\P_\perp,\max}:= \max_t \|\P_\perp{}'\bm\Sig_{v,t}\P\|,\ \lambda_{v,\max}^+:=\max_t \|\bm\Sigma_{v,t}\|.
\]
It is easy to see that $\lambda_{v,\P,\P_\perp,\max} \le  \lambda_{v,\rest,\max}^+$. Also, $\lambda_{v,\rest,\max}^+ \le \lambda_{v,\max}^+$,  $\lambda_{v,\P,\avg}^- \le \lambda_{v,\max}^+$.

\item The following factor (noise-to-signal ratio) of uncorrelated noise will used at various places in our results:
\[
\nois: = \frac{\lambda_{v,\max}^+}{\lambda^-_{\avg}}
\]

\item We also define ``effective dimension''  for the uncorrelated noise as
\[
r_v := \max_t \|\vp_t\|^2/\lambda_{v,\max}^+
\]
\item Define $\Sig_{w,t} = \E[\wt\wt{}']$, $\Sigwb = \frac{1}{\tmaxpca}\sum_t\Sig_{w,t}$ and $\Sig_{w,l,t} := \E[\lt\wt{}' + \wt\lt{}']$, $\Sigw = \frac{1}{\tmaxpca}\sum_t\Sig_{w,l,t}$ and $\bar{\Sig}_{w,\rest} := \Sigw - \P\P{}'\Sigw\P\P{}'$.
\item Let $\Phat$ denote the matrix of top-$r$ eigenvectors of the sample-covariance matrix, $\D = \sum_t \yt \yt{}'$.
\een
%We assume that $\lambda_v^+$ and $\lambda^+$ are at most constant ($O(1)$) with $n$.
\label{def1}
\end{definition}

We have the following result.
\begin{theorem}
%Given an $1 > \varepsilon_\SE  > 0$ and
Given data vectors $\yt := \lt + \wt + \vp_t$ where $\wt = \M_t \lt$, and $\vp_t$ and $\lt$ are uncorrelated, i.e., $\E[\lt\vp_t{}'] = 0$. Assume that there exist constants $\bz <1$, $q < 2$, and the  matrices $\M_t$ can be decomposed as $\M_t = \M_{2,t} \M_{1,t}$  with
$\M_{1,t}$ being such that
\bea
\max_t \|\M_{1,t} \P\|_2 := q <2
\eea
and
$\M_{2,t}$ being such that $\|{\bm{M}_{2,t}}\|_2 \le 1$ and %for any $\tmaxpca > \tmaxpca_w:= ,
\bea
% \left\|\frac{1}{\tmaxpca} \sum_{t =1}^\tmaxpca {\bm{M}_{2,t}} \bm{A}_t {\bm{M}_{2,t}}' \right\|_2  \le \bz \max_{t \in [1,\tmaxpca]} \|\bm{A}_t\|.
 \left\|\frac{1}{\tmaxpca} \sum_{t =1}^\tmaxpca {\bm{M}_{2,t}} {\bm{M}_{2,t}}' \right\|_2  \le \bz
\label{M2t_bnd}
\eea
\label{Mt_cond}
Then we have
\begin{align}
\label{eq:pca_thm}
&\SE(\Phat, \P) \nn \\ 
&\leq \frac{\frac{\lambda_{v,\P,\P_\perp,\max}}{\lambda^-_{\avg} } + \sqrt{\bz} (q + q^2) f + \epsbnd }{1  -  \frac{\lambda_{v,\rest,\max}^+ - \lambda_{v,\P,\avg}^-}{\lambda^-_{\avg}}  - 2 \sqrt{\bz} (2q + q^2) f  - \epsbnd - \epsden}
%\\ &\leq \frac{\frac{\lambda_{v,\P,\P_\perp,\max}}{\lambda^-_{\avg} } + 3\sqrt{\bz} q f + \epsbnd }{1  -  \frac{\lambda_{v,\rest,\max}^+ -  \lambda_{v,\P,\avg}^-}{\lambda^-_{\avg}}  - 3 \sqrt{\bz} q f  - \epsbnd - \epsden}
\end{align}
%\begin{align*}
%\SE(\Phat, \P) &\leq {\text{bias-error}} + {\text{statistical-error}}, \ \ \text{where} \\
%\underbrace{\SE(\Ptil, \P)}_{\color{red}\text{bias error}} &\leq \frac{\frac{\lambda_{v, \P, \P_{\perp}}}{\lambda^- + \lambda_{v, \P}^-} + 2 \sqrt{\bz}qf}{1 - \frac{\lambda_{v, \rest}^+ }{\lambda^- + \lambda_{v, \P}^-} - 6 \sqrt{\bz}qf}
%\end{align*}
where
$\epsbnd$ and $\epsden$ depends on the statistical properties of the data and noise and we have
%\begin{align*}
%\end{align*}
%and $\epsbnd$ depends on the data and noise distribution, and in particular we have that
\begin{enumerate}
\item
%Assume that $\at$'s are zero-mean, mutually independent, element-wise bounded r.v.'s and have a diagonal covariance $\Lam_t$. Element-wise bounded-ness implies that there exists a numerical constant, $\eta$, such that, for all $t$,
%$
%\max_{j}  \max_t [( \at)_j^2/\lambda_j(\Lam_t)] \le \eta
%$. For example, if $\at$'s are uniformly distributed, then $\eta = 3$. Throughout this paper, $\eta$ will be treated as a numerical constant.
Assume that $\at$'s are bounded s.t. $\|\at\|_2^2 \leq \eta r \lambda^+$ for a numerical constant $\eta$. And $\vp_t$'s are zero-mean, mutually independent, bounded r.v.'s (see last item of Definition \ref{def1}), have a diagonal covariance $\Sig_v$,  and are uncorrelated with $\at$'s. Then, %we have %with probability at least $1 - 10n^{-10}$,
\begin{align*}
\epsbnd &:= C \sqrt{\eta} \max \left( qf \sqrt{\frac{r \log n}{\tmaxpca}} , \sqrt{\nois f}  \sqrt{\frac{r_v \log n}{\tmaxpca}}\right)  \\
\epsden &:= c \eta f \sqrt{\frac{r\log n}{\tmaxpca}}
\end{align*}
as long as the denominator of \eqref{eq:pca_thm} is positive.
%\item Instead of $\at$'s being element-wise bounded, assume that $\at$'s are bounded as $\|\at\|_2^2 \leq \eta r \lambda^+$ for a numerical constant $\eta$ and assume that all other conditions of the first item hold. Then,
%\begin{align*}
%\epsbnd &:= C \sqrt{\eta} \max \left( qf \sqrt{\frac{r \log n}{\tmaxpca}} , \sqrt{\nois f}  \sqrt{\frac{r_v \log n}{\tmaxpca}}\right)  \\
%\epsden &:= c \eta f \sqrt{\frac{r\log n}{\tmaxpca}}
%\end{align*}
\item If $\at$'s are sub-Gaussian r.v.'s with sub-Gaussian norms bounded by $C \sqrt{\lambda^+}$ and similarly, $\vp_t$'s are sub-Gaussian r.v.'s with sub-Gaussian norms bounded by $C \sqrt{\lambda^+_v}$ and are uncorrelated with $\at$'s.%
Then with probability at least $1 - 10 \exp(-cn)$,
\begin{align*}
\epsbnd &:= C \sqrt{\nois f} \sqrt{\frac{n}{\tmaxpca}} \\
\epsden &:= c \eta f \sqrt{\frac{r + \log n}{\alpha}}
\end{align*}
\end{enumerate}

Furthermore, when the rank is unknown, we can compute $\hat{r}$ as
\bea
\hat{r}:= \arg \min \{j: \lambda_j(\D)  \ge 0.5  \lambda^-_{\avg} \}
\label{estim_r_1}
\eea
Then, with probability at least $1 - 10n^{-10}$, $\hat{r} = r$

\label{mainthm}
\end{theorem}

\subsection{Proof}
The overall proof relies on a systematic application of the standard Davis Kahan $\sin\theta$ theorem \cite{davis_kahan} summarized here.

\begin{lem}[Davis-Kahan $\sin \theta$ theorem]\label{sintheta2}
Let $\D_0$ be a Hermitian matrix whose span of top $r$ eigenvectors equals $\Span(\P)$. Let $\D$ be the Hermitian matrix with top $r$ eigenvectors  $\Phat$. Then,
\begin{align}
\SE(\Phat,\P) &\le \frac{\|(\D-\D_0)\P\|}{\lambda_r(\D_0) - \lambda_{r+1}(\D)}   \nn \\
&\le  \frac{\|\D-\D_0\|}{\lambda_r(\D_0) - \lambda_{r+1}(\D_0) - \lambda_{\max}(\D-\D_0)}
%\label{sintheta_bnd}
\label{sintheta_bnd_2}
\end{align}
as long as the denominator is positive. The second inequality follows from the first using Weyl's inequality.
\end{lem}

Recall that we are provided with observations $\yt = \lt + \wt + \vp_t$. Thus, $\Sig_t = \E[\yt \yt{}'] = \P\Lam_t\P{}' + \Sig_{v,t} + \Sig_{w,t} + \Sig_{w,l,t}$ where $\Sig_{w,t} = \M_t\P \Lam_t \P{}'\M_t{}'$ and $\Sig_{w,l,t} = \P\Lam_t \P{}'\M_t{}' + \M_t \P\Lam_t \P{}'$. This follows because the matrices $\M_t$ are deterministic but unknown. Since the covariance is non-stationary, we define the time-averaged covariances as $\Lamb = \frac{1}{\tmaxpca} \sum_t \Lam_t$, $\Sigb = \frac{1}{\tmaxpca}\sum_t \Sig_t$ $\Sigvb = \frac{1}{\tmaxpca} \sum_t \Sig_v$, $\Sigwb = \frac{1}{\tmaxpca} \sum_t \Sig_w$, $\Sigw = \frac{1}{\tmaxpca}\sum_t \Sig_{w,l,t}$. Then it is easy to see that $\Sigvb = (\P \P{}' + \P_{\perp} \P_{\perp}{}') \Sigvb (\P \P{}' + \P_{\perp} \P_{\perp}{}')$. Similarly, we can obtain expressions for $\Sigwb$ and $\Sigw$. After some simple algebra, it follows that we can define $\bm{D}_0 = \P[\frac{1}{\tmaxpca}\sum_t\at\at{}' + \P{}'(\Sigvb +\Sigwb + \Sigw) \P]\P{}'$ to be a Hermitian matrix with $\Phat$ as the top $r$ eigenvectors, and $\bm{D} = \frac{1}{\tmaxpca}\sum_t \yt \yt{}'$ to be a Hermitian matrix with $\Phat$ as the top $r$ eigenvectors.

Now, we apply the $\sin\theta$ theorem %and rewrite $\D - \D_0$ as $ \E[\D - \D_0] + (\D - \D_0 - \E[\D - \D_0])$
\begin{align*}
&\SE(\Phat, \P) \leq \frac{\|(\D - \D_0)\P\|}{\lambda_{r}(\bm{D}_0) - \lambda_{r+1}(\bm{D})} \\
&\leq \frac{\|(\E[\D - \D_0])\P\| + \|(\D - \D_0 - \E[\D - \D_0])\P\|}{\lambda_{r}(\bm{D}_0) - \lambda_{r+1}(\bm{D})} \\
&\leq \frac{\|\P_{\perp}\P_{\perp}{}'( \Sigvb +\Sigwb + \Sigw) \P\|+\|\D - \D_0 - \E[\D - \D_0]\|}{\lambda_{r}(\bm{D}_0) - \lambda_{r+1}(\bm{D})} \\
&:= \frac{\|\P_{\perp}\P_{\perp}{}'( \Sigvb +\Sigwb + \Sigw) \P\|+ \|T_1\|}{\lambda_{r}(\bm{D}_0) - \lambda_{r+1}(\bm{D})}
\end{align*}
using Weyl's inequality, and observing that $\P{}' (\Sigw + \Sigwb)\P$ is a positive semidefinite matrix we have that
\begin{align*}
\lambda_{r}(\D_0) &\geq \lambda_r(\Lamb) + \lambda_{\min}(\P{}' \Sigvb \P) + \lambda_{\min}(\P{}'(\Sigw +\Sigwb) \P)  \\
&+ \lambda_{\min}\left(\frac{1}{\tmaxpca}\sum_t \at\at{}'- \Lamb\right) \\
&\geq \lambda^-_{\avg} + \lambda_{v, \P, \min}^- - \norm{\frac{1}{\tmaxpca}\sum_t\at\at{}' - \Lamb}
\end{align*}
we will bound the last term using Lemma \ref{hp_bnds}.

Furthermore,
\begin{align}\label{eq:weyl_bias}
\lambda_{r+1}(\D) &\leq \lambda_{r+1}(\D_0) + \lambda_{\max}(\E[\D -\D_0]) + \|T_1\| \nn \\
&= 0 + \lambda_{\max}(\bar{\Sig}_{v,\rest} + \bar{\Sig}_{w, \rest} + \bar{\Sig}_{w,l,\rest}) + \|T_1\|  \nn \\
&\leq \lambda_{\max}(\bar{\Sig}_{v,\rest}) + \lambda_{\max}(\bar{\Sig}_{w,\rest}) + \lambda_{\max}(\bar{\Sig}_{w,\rest}) + \|T_1\| \nn \\
&\leq \lambda_{v,\rest,\max}^+ + 2\|\Sigwb\| + 2\|\Sigw\| + \|T_1\|
\end{align}
Consider the numerator term
\begin{align*}
&\|\P_{\perp}\P_{\perp}{}'( \Sigvb + \Sigwb + \Sigw) \P\|  \\
&\leq \|\P_{\perp}\P_{\perp}{}'\Sigvb\P\|  + \|\P_{\perp}\P_{\perp}{}'\Sigwb\P\| + \|\P_{\perp}\P_{\perp}{}'\Sigw\P\| \\
&\leq \lambda_{v, \P, \P_{\perp}, \max}+ \|\P_{\perp}\P_{\perp}{}'\Sigwb\P\| + \|\P_{\perp}\P_{\perp}{}'\Sigw\P\|
\end{align*}
In the last term of the r.h.s. above, notice that due to the projection matrix $\P_{\perp}\P_{\perp}{}'$, the first term of $\Sigw$ is nullified, and hence we need to consider only $\Sigwb$ and the second term of $\Sigw$. Both these terms are bounded using Cauchy-Schwartz inequality for matrices as follows. Recall that $\M_t = \M_{2,t} \M_{1,t}$ with $\|\frac{1}{\tmaxpca} \sum_t \M_{2,t} \M_{2,t}{}'\| \leq \bz$ and $\|\M_{1,t} \P\| \leq q < 2$. Thus,
\begin{align}
&\norm{\frac{1}{\tmaxpca} \sum_t \M_t \P \Lam_t \P'\M_{1,t}{}' \M_{2,t}{}'}_2^2 \nn \\
 & \le  \norm{\frac{1}{\tmaxpca} \sum_t \M_{t} \P \Lam_t \P'\M_{1,t}{}'\M_{1,t}\P \Lam_t \P'\M_{t}{}'}_2  \norm{\frac{1}{\tmaxpca} \sum_t \M_{2,t} \M_{2,t}{}'}_2 \nn \\
& \le  \max_t \|\M_{t}\P \Lam_t \P'\M_{1,t}{}' \|_2^2  \ \bz \le  (q^2 \lambda^+_{\max})^2 \bz.
%\label{bnd_avg_sig_noise_cor_bnd_2}
\end{align}
The cross term can be bounded in a similar fashion
\begin{align}
&\norm{\frac{1}{\tmaxpca} \sum_t \M_{2,t} \M_{1,t} \P \Lam_t \P'}_2^2 \nn \\
 & \le  \norm{\frac{1}{\tmaxpca} \sum_t \P \Lam_t \P'\M_{1,t}{}'\M_{1,t}\P \Lam_t \P'}_2  \norm{\frac{1}{\tmaxpca} \sum_t \M_{2,t} \M_{2,t}{}'}_2 \nn \\
& \le \max_t \|\M_{1,t}\P \Lam_t \P'\|_2^2 \ \bz \le  (q \lambda^+_{\max})^2 \bz.
%\label{bnd_avg_sig_noise_cor_bnd_1}
\end{align}
From these, it is easy to see that
\begin{align*}
\|\P_{\perp} \P_{\perp}{}'\Sigw\P\| + \|\P_{\perp} \P_{\perp}{}'\Sigwb\P\| \leq q \lambda^+ (1 + q) \sqrt{\bz} \leq 3 \sqrt{\bz}q\lambda^+_{\max}
\end{align*}
Finally for the denominator,
\begin{align*}
\|\Sigwb\| + \|\Sigw\| \leq q \lambda^+_{\max} (2 + q) \sqrt{\bz} \leq 4 \sqrt{\bz}q\lambda^+_{\max}
\end{align*}

Using these bounds, we conclude that
\begin{strip}
\begin{align*}
\SE(\Phat, \P) 
 &\leq \frac{\lambda_{v, \P, \P_{\perp}, \max} + 3 \sqrt{\bz}q\lambda^+_{\max} + \|T_1\|}{\lambda^-_{\avg} + \lambda_{v,\P,\avg}^- - \lambda_{v, \rest,\max}^+ - 8 \sqrt{\bz}q\lambda^+_{\max} - \norm{\frac{1}{\tmaxpca}\sum_t \at\at{}' - \Lamb} - \|T_1\|} \\
&= \frac{\frac{\lambda_{v, \P, \P_{\perp},\max} + 3 \sqrt{\bz}q\lambda^+_{\max}}{\lambda^-_{\avg} + \lambda_{v,\P,\avg}^-} + \frac{\|T_1\|}{\lambda^-_\avg}}{1 - \frac{\lambda_{v, \rest,\max}^+ + 8 \sqrt{\bz}q\lambda^+_{\max}}{\lambda^-_{\avg} + \lambda_{v,\P,\avg}^-} - \frac{\norm{\frac{1}{\tmaxpca}\sum_t \at\at{}' - \Lamb} + \|T_1\|}{\lambda^-_\avg}}\\
&\leq \frac{\frac{\lambda_{v, \P, \P_{\perp}, \max}}{\lambda^-_{\avg} + \lambda_{v, \P, \min}^-} + 3 \sqrt{\bz}qf  + \frac{\|T_1\|}{\lambda^-_\avg}}{1 - \frac{\lambda_{v, \rest,\max}^+ }{\lambda^-_{\avg} + \lambda_{v,\P,\avg}^-} - 8 \sqrt{\bz}qf - \frac{\norm{\frac{1}{\tmaxpca}\sum_t \at\at{}' - \Lamb} + \|T_1\|}{\lambda^-_\avg}}
\end{align*}
\end{strip}

To bound $\|T_1\|_2$ and $\|\frac{1}{\alpha} \sum_t \at \at' - \Lamb\|_2$, we use concentration bounds from the Lemma \ref{hp_bnds}. Notice that
\begin{strip}
\begin{align*}
T_1 &= \frac{1}{\tmaxpca}\sum_t(\vp_t \vp_t{}' - \E[\vp_t\vp_t{}'])] + \frac{1}{\tmaxpca}\sum_t(\wt \wt{}' - \E[\wt\wt{}'])] \\
&+\frac{1}{\tmaxpca}\sum_t(\lt \wt{}' - \E[\lt\wt{}'])] + \frac{1}{\tmaxpca}\sum_t(\wt \lt{}' - \E[\wt\lt{}'])] + \frac{1}{\tmaxpca}\sum_t \lt \vp_t{}' + \frac{1}{\tmaxpca}\sum_t \wt \vp_t{}'  \\
%\end{align*}
%and thus
%\begin{align*}
&\implies \|T_1\| \leq \norm{\frac{1}{\tmaxpca}\sum_t(\vp_t \vp_t{}' - \E[\vp_t\vp_t{}'])]} + \norm{\frac{1}{\tmaxpca}\sum_t(\wt \wt{}' - \E[\wt\wt{}'])]} \\
&+ 2\norm{\frac{1}{\tmaxpca}\sum_t(\lt \wt{}' - \E[\lt\wt{}'])]} + \norm{\frac{1}{\tmaxpca}\sum_t \lt \vp_t{}'} + \norm{\frac{1}{\tmaxpca}\sum_t \wt \vp_t{}'} \\
&\leq c\sqrt{\eta}  \nois \sqrt{\frac{r_v \log n}{\tmaxpca}} \lambda^-_{\avg} + c\sqrt{\eta} q^2  f  \sqrt{\frac{r \log n}{\tmaxpca}}   \lambda^-_{\avg} + c\sqrt{\eta} q f  \sqrt{\frac{r \log n}{\tmaxpca}}     \lambda^-_{\avg}  \\
&+ c\sqrt{\eta} \sqrt{\nois f} \sqrt{\frac{ \max(r_v, r) \log n}{\tmaxpca}} \lambda^-_{\avg}  + c\sqrt{\eta} q \sqrt{\nois f} \sqrt{\frac{ \max(r_v, r) \log n}{\tmaxpca}} \lambda^-_{\avg} \\
&\leq C \sqrt{\eta} \max \left( qf \sqrt{\frac{r \log n}{\tmaxpca}} , \sqrt{\nois f}  \sqrt{\frac{r_v \log n}{\tmaxpca}}\right)  \lambda^-_{\avg} := \epsbnd\lambda^-_{\avg}
\end{align*}
\end{strip}
where the last line follows from using $q^2 \leq 2q $, $\nois \leq f$, and $r \leq r_v$. The bound on $\|\frac{1}{\alpha} \sum_t \at \at' - \Lamb\|_2$ follows directly from the first item of Lemma \ref{hp_bnds}.

\subsubsection{Sub-Gaussian data and noise}
For the setting where the data and noise are drawn from a sub-Gaussian distribution, the only thing that changes is the bounds on ``statistical errors''. We will need the following result. Its proof follows from Lemma \cite[Theorem 4.6.1]{versh_book} with one change: since the matrix is not symmetric, we use $\|\L \V{}'\| = \max_{\bm{z}_1,\bm{z}_2} |\bm{z}_1{}'\L \V{}' \bm{z}_2|$.

\begin{lem}\label{lem:cross_subg}
Let $\bx_i$, $i=1,2,\dots,N$, and $\by_i, i=1,2,\dots, N$ be zero mean sub-Gaussian random vectors with sub-Gaussian norms bounded by $K_x$ and $K_y$ respectively. Each $\bx_i, \by_i$ is in $\Re^n$. Also $\{\bx_i, \by_i\}$, $i=1,2,\dots, N$ are mutually independent.
Then,
%where $\bx_i$'s are mutually independent, zero-mean, sub Gaussian random vectors in $\Re^n$ with sub Gaussian norm bounded by $K_x$ and $\by_i$'s are mutually independent, zero-mean, sub Gaussian random vectors in $\Re^n$ with sub Gaussian norm bounded by $K_y$ %. Note that the pairs $\{\bx_i, \by_i\}$ are not necessarily independent. Then,
\begin{align*}
%\Pr\left(\norm{\frac{1}{N} \sum_i \bx_i \by_i{}' - \E \left[\frac{1}{N} \sum_i \bx_i \by_i{}'\right]} \le t \right) \geq 1 - 2 \exp \left(n \log 9 - \frac{t^2 N}{16c(K_x^2 + K_y^2)} \right)
&\Pr\left(\norm{\frac{1}{N} \sum_i \bx_i \by_i{}' - \E \left[\frac{1}{N} \sum_i \bx_i \by_i{}'\right]} \le t \right) \\
&\geq 1 - 2 \exp \left(n \log 9 - \frac{t^2 N}{16c(K_xK_y)} \right)
\end{align*}
\end{lem}

Using the above result, we get the following bounds for the statistical errors.

\begin{lem}\label{hp_bnds_subg}
Under conditions of Theorem \ref{thm1} if the data and noise follow the sub-Gaussian model, with probability at least $1 - 2 \exp(-cn)$
\begin{align*}
&\norm{\frac{1}{\tmaxpca} \sum_t \lt \vp_t{}' }_2 \leq C \sqrt{\nois f} \sqrt{\frac{n}{\tmaxpca}} \lambda^-_{\avg}\\
&\norm{\frac{1}{\tmaxpca} \sum_t \vp_t \vp_t{}' - \frac{1}{\tmaxpca}\E\left[\sum_t \vp_t \vp_t{}'\right]}_2 \leq C \sqrt{\eta} \nois \sqrt{\frac{n}{\tmaxpca}} \lambda^-_{\avg}\\
&\norm{\frac{1}{\tmaxpca} \sum_t \wt \vp_t{}'}_2 \leq  C \sqrt{\eta} q \sqrt{\nois f}  \sqrt{\frac{n}{\tmaxpca}} \lambda^-_{\avg}
\end{align*}
\end{lem}
\begin{proof}
Consider the $\lt \vp_t{}'$ term. Apply Lemma \ref{lem:cross_subg} with $\bx_t = \lt$, $\by_t = \vp_t$,  $N \equiv \tmaxpca$.  Recall that $\E[\lt \vp_t{}'] = 0$. Furthermore, for bounded r.v.'s the sub-Gaussian norm is equal to the bound thus $K_x = c\sqrt{\lambda^+_{\max}}$ and $K_y = c\sqrt{\lambda^+_{v,\max}}$, thus $K_x K_y = c \sqrt{\lambda^+_{\max}  \lambda^+_{v, \max}}$ %\le c \max(\lambda^+,\lambda_v^+)$.
Set $t = \epsilon_{0, v} \lambda^-_{\avg}$ with $\epsilon_{0,v}= c \sqrt{\nois f} \sqrt{\frac{n}{\tmaxpca}}$.
Then with probability at least $1- 2\exp(-c n)$
\begin{align*}
\norm{\frac{1}{\tmaxpca} \sum_t \lt \vp_t{}'}_2 \leq c \sqrt{\nois f} \sqrt{\frac{n}{\tmaxpca}} \lambda^-_{\avg}
\end{align*}
%Similar ideas can be applied to $\vp_t \vp_t{}'$ and $\wt \vp_t{}'$ terms.
The proof for $\vp_t\vp_t{}'$ and  $\wt\wt{}'$ follows exactly in the same way.
\end{proof}

Observe that the bounds on the other terms follow in exactly the same way.

\begin{remark}[Bias and Statistical Error]
In Theorem \ref{mainthm}, notice that \eqref{eq:pca_thm} can also be written as
\begin{strip}
\begin{align*}
\SE(\Phat, \P) \leq \frac{1}{\text{denominator}}\cdot \left(\underbrace{\frac{\lambda_{v,\P,\P_\perp,\max}}{\lambda^-_{\avg} + \lambda_{v,\P,\avg}^-} + \sqrt{\bz} (q + q^2) f}_{\cred{Bias-Error}} + \underbrace{\epsbnd}_{\cred{Stat-Error}} \right)
\end{align*}
\end{strip}
where the first term denotes the bias error. This quantifies the {\em distance} between the desired subspace, and the top-$r$ eigenvectors of the population covariance matrix. The second term is the statistical error which quantifies the {\em distance} between the top-$r$ eigenvectors of the population covariance and the sample covariance. The statistical error can be made arbitrarily small by increasing the number of samples, $\tmaxpca$ whereas the bias error is a function of the data-noise model. It is not possible to completely de-couple the two terms, due to a technical reason. Doing this will come at an additional factor of $1/\epsilon^2$ when applied to NORST.
\end{remark}

\section{Theorems we use and Proofs of Auxiliary Lemmas}\label{app:concm}
%First, we provide the proof of Lemma \ref{lem:sumprinang}.

\begin{proof}[Proof of Lemma \ref{lem:sumprinang}]
The proof of upper bound follows from triangle inequality as
\begin{align*}
&\SE(\Aa, \Ca) = \norm{(\I - \Aa \Aa{}') \Ca} \\
&= \norm{(\I - \Aa \Aa{}')(\I - \Ba \Ba{}' + \Ba \Ba{}') \Ca} \\
&\leq \norm{(\I - \Aa \Aa{}')(\I - \Ba \Ba{}')\Ca} + \norm{(\I - \Aa \Aa{}') \Ba \Ba{}' \Ca} \\
&\leq \norm{(\I - \Aa \Aa{}')} \SE(\Ba, \Ca) + \SE(\Aa, \Ba) \norm{\Ba{}' \Ca} \\
&\leq \Delta_1 + \Delta_2
\end{align*}
We now obtain the lower bound
\begin{align*}
&\SE(\Aa, \Ca) = \norm{(\I - \Aa \Aa{}') \Ca} \\
&= \norm{(\I - \Aa \Aa{}' - \Ba \Ba{}' + \Ba \Ba{}') \Ca} \\
&\geq \norm{(\I - \Ba \Ba{}')\Ca} - \norm{ (\Ba \Ba{}' - \Aa \Aa{}')  \Ca} \\
&\geq \SE(\Ba, \Ca)  - \norm{\Ba \Ba{}' - \Aa \Aa{}'} \\
&\geq \SE(\Ba, \Ca) - 2 \SE(\Aa, \Ba)
\end{align*}

\end{proof}

%We need the following results for proving Lemma \ref{lem:concm}.

%We use the following preliminaries to prove the main Lemma.
%Cauchy-Schwartz for sums of matrices says the following\cite{rrpcp_perf}.
\begin{theorem}[Cauchy-Schwartz for sums of matrices \cite{rrpcp_perf}] \label{CSmat}
For matrices $\bm{X}$ and $\bm{Y}$ we have
\begin{eqnarray}\label{eq:csmat}
\norm{\frac{1}{\alpha} \sum_t \bm{X}_t \bm{Y}_{t}{}'}^2 \leq \norm{\frac{1}{\alpha} \sum_t \bm{X}_t \bm{X}_t{}'} \norm{\frac{1}{\alpha} \sum_t \bm{Y}_t \bm{Y}_t{}'}
\end{eqnarray}
\end{theorem}
The following theorem is adapted from \cite{tail_bound}.
\begin{theorem}[Matrix Bernstein \cite{tail_bound}]\label{thm:matrix_bern}
Given an $\alpha$-length sequence of $n_1 \times n_2$ dimensional random matrices and a r.v. $X$. Assume the following holds. For all $X \in \mathcal{C}$, (i) conditioned on $X$, the matrices $\Z_t$ are mutually independent, (ii) $\mathbb{P}(\norm{\Z_t} \leq R | X)  = 1$,  and (iii) $\max\left\{\norm{\frac{1}{\alpha}\sum_t \ep{\left[\Z_t{}'\Z_t | X\right]}},\ \norm{\frac{1}{\alpha}\sum_t \ep{\left[\Z_t\Z_t{}' | X\right]}}\right\} \le \sigma^2$. Then, for an $\epsilon > 0$ and for all $X \in \mathcal{C}$,
\begin{align}
\mathbb{P}\left(\norm{\frac{1}{\alpha} \sum_t \Z_t} \leq \norm{\frac{1}{\alpha} \sum_t \ep{\left[\Z_t|X\right]}} + \epsilon\bigg|X\right) \nn \\ 
 \geq 1 - (n_1 + n_2) \exp\left(\frac{-\alpha\epsilon^2}{2\left(\sigma^2 + R \epsilon\right)} \right).
\end{align}
\end{theorem}

The following theorem is adapted from \cite{versh_book}.
\begin{theorem}[Sub-Gaussian Rows \cite{versh_book}]\label{thm:versh}
Given an $N$-length sequence of sub-Gaussian random vectors $\bm{w}_i$ in $\mathbb{R}^{n_w}$, an r.v $X$, and a set $\mathcal{C}$. Assume the following holds. For all $X \in \mathcal{C}$, (i) $\bm{w}_i$ are conditionally independent given $X$; (ii) the sub-Gaussian norm of $\bm{w}_i$ is bounded by $K$ for all $i$. Let $\bm{W}:=[\bm{w}_1, \bm{w}_2, \dots, \bm{w}_N]{}'$.
Then for an $\epsilon \in (0, 1)$ and for all $X \in \mathcal{C}$
\begin{align}
\mathbb{P}\left(\norm{\frac{1}{N}\bm{W}{}'\bm{W} - \frac{1}{N}\ep{\left[\bm{W}{}'\bm{W} | X \right]}} \leq \epsilon \bigg| X\right) \nn \\ 
\geq 1 - 2\exp\left({n_w} \log 9 - \frac{c \epsilon^2 N}{4K^4}\right).
\end{align}
\end{theorem}

\section{Obtaining a result similar to that of \cite{rrpcp_dynrpca} for NORST}\label{sec:proof_reprocs-pca-mc}

It is possible to relax the lower bound on outlier magnitudes if not all of the subspace directions change at a given subspace change time. Suppose that only $r_\ch < r$ directions change. When $r_\ch=1$, we recover the guarantee of \cite{rrpcp_dynrpca} but for NORST (which is a simpler algorithm than s-reprocs).
%we impose a slightly more stringent model on how the subspace changes. Furthermore, this result is the model considered in s-ReProCS \cite{rrpcp_dynrpca} and as we show below, our result recovers their result. Concretely, if the subspace changes such that only $r_\ch \ll r$ directions change at each subspace change time, i.e., under the same notation of Theorem \ref{thm1} the subspace changes as follows, or all $j$,

Let $\P_{j-1, \fx}$ denote a basis for the fixed component of $\P_{j-1}$ and let $\P_{j-1,\ch}$ denote a basis for its changing component. Thus,
$\P_{j-1} \R = [ \P_{j-1,\fx}, \P_{j-1,\ch}]$, where $\bm{R}$ is a $r \times r$ rotation matrix. %$\P_{j-1, \fx}$ is the ``fixed component'' with dimensions $n \times (r - r_\ch)$, $\P_{j-1, \ch}$ is the ``changing component'' with dimensions $n \times r_\ch$. and $\bm{R}$ is a $r \times r$ rotation matrix. Further
We have
\begin{align}\label{eq:rchdef1}
\P_j = [\P_{j-1,\fx}, \P_{j,\chd}]
\end{align}
where $\P_{j, \chd}$ is the changed component and has the same dimension as $\P_{j-1, \ch}$. Thus,
\begin{align}\label{eq:rchdef2}
\SE(\P_{j-1},\P_j) = \SE( \P_{j-1,\ch}, \P_{j,\chd})
\end{align}
and so $\Delta = \max_j \SE(\P_{j-1},\P_j) = \max_j \SE( \P_{j-1,\ch}, \P_{j,\chd})$.
Let $\lambda_{\ch}^+$ denote the largest eigenvalue along any direction in $\P_{j,\chd}$.
\begin{corollary}\label{cor:rch}
In Algorithm \ref{algo:auto-reprocs-pca}, replace line 17 by $\Phat_{(t)} \leftarrow \basis(\Phat_{j-1}, \Phat_{j, k})$. For basis matrices $\P_1, \P_2$, we use $\P = \basis(\P_1, \P_2)$ to mean that $\P$ is a basis matrix with column span equal to the column span of $[\P_1, \P_2]$.
Assume that  \eqref{eq:rchdef1} and \eqref{eq:rchdef2} hold. Also assume that the conditions of Theorem \ref{thm1} holds with the lower bound on $\xmint$ relaxed to $\xmint \ge C (\zz \sqrt{\eta (r - r_\ch) \lambda^+} + (\zz + \Delta) \sqrt{\eta r_\ch \lambda_\ch^+})$.
Then, all conclusions of Theorem \ref{thm1} hold.% with the same probability.
\end{corollary}

\begin{proof}[Proof of Corollary \ref{cor:rch}]
The proof is very similar to that of Theorem \ref{thm1}. The only changes occur in the \\
\emph{(a) Projected CS step}. With the subspace change model, we define
$
\lt = \P_{(t)} \at :=
\begin{bmatrix} \P_{j-1, \fx} & \P_{j, \chd} \end{bmatrix}
\begin{bmatrix}
\atf \\
\atr
\end{bmatrix}
$
where $\atf$ is a $(r - r_\ch) \times 1$ dimensional vector and $\atr$ is a $r_\ch \times 1$ dimensional vector. %This analysis below clarifies why the change in Algorithm \ref{algo:auto-reprocs-pca} is needed. %This helps in getting a tighter bound on the error incurred in the sparse recovery step.
In the first $\alpha$ frames after the $j$-th subspace changes (or, the $j$-th subspace change is detected in the automatic case), recall that $\Phat_{(t)} = \Phat_{j-1}$. Thus, $\SE(\Phat_{(t)}, \P_{j-1, \fx}) =
\SE(\Phat_{j-1}, \P_{j-1, \fx}) \leq \SE(\Phat_{j-1}, \P_{j-1}) \leq \zz$ and so, the error can be bounded as
\begin{align*}
\norm{\bpsi \lt} &\leq \norm{\bpsi \P_{j-1, \fx} \atf} + \norm{\bpsi \P_{j, \chd} \atr} \\
&\leq \zz \sqrt{\eta (r - r_\ch) \lambda^+} + (\zz + \SE(\P_{j-1}, \P_j)) \sqrt{\eta r_\ch \lambda_\ch^+}
\end{align*}
%The second term follows using Lemma \ref{lem:sumprinang} with $\Aa = \Phat_{j-1}$, $\Ba = \P_{j-1}$ and $\Ca = \P_{j}$.
In the second $\alpha$ frames, have $\Phat_{(t)} = \basis(\Phat_{j-1}, \Phat_{j,1})$. Thus $\SE(\Phat_{(t)}, \P_{j-1,\fx}) \le
\SE(\Phat_{j-1}, \P_{j-1, \fx}) \leq \SE(\Phat_{j-1}, \P_{j-1}) \leq \zz$ and $\SE(\Phat_{(t)},\P_{j, \chd}) \le  \SE(\Phat_{j,1}, \P_{j, \chd}) \leq \SE(\Phat_{j,1}, \P_{j}) \leq 0.3 \cdot (\zz + \SE(\P_{j-1}, \P_j))$. Thus, the error in the sparse recovery step in the interval after the  first subspace update is  performed is given as
\begin{align*}
\norm{\bpsi \lt} \leq \zz \sqrt{\eta (r - r_\ch) \lambda^+} + 0.3 \cdot (\zz + \SE(\P_{j-1}, \P_j)) \sqrt{\eta r_\ch \lambda_\ch^+}
\end{align*}
The rest of the proof follows as before.
The error after the $k$-th subspace update is also bounded using the above idea.

%and thus satisfies the minimum outlier magnitude bound. Similar to the second $\alpha$ frames, the error in the $k$-th subspace update, i.e., $t \in [\that_j + k \alpha, \that_j + (k+1)\alpha)$, $\SE(\Phat_{j,k}, \P_{j, \chd}) \leq 0.3^k (\zz + \SE(\P_{j-1}, \P_j))$. The proof of the remaining steps follow in exactly the same way as before.

\emph{(b) Subspace Detection step}:
The proof of the subspace detection step follows exactly analogous to Lemma \ref{lem:sschangedet}. One minor observation is noting that $\SE(\P_{j-1}, \P_J) = \SE(\P_{j-1, \ch}, \P_{j, \chd})$ in the proof of part (a) of Lemma \ref{lem:sschangedet}. The rest of the argument is exactly the same.
\end{proof}
