# Supplementary material for: Fast Robust Subspace Tracking via PCA in Sparse Data-Dependent Noise
Source: arXiv:2006.08030 source file (2020-12-04)
Supplement: Supplementary file 2 [file norst_supp_sims.tex]

\section{Synthetic Experiments Extra Details}
All time comparisons are performed on a Desktop Computer with Intel$^{\textsuperscript{\textregistered}}$ Xeon E$3$-$1240$ $8$-core CPU @ $3.50$GHz and $32$GB RAM and all synthetic data experiments are averaged over $100$ independent trials. The codes are available at \url{https://github.com/praneethmurthy/NORST}. 
\subsubsection{Algorithm Parameters}
For $l_1$ minimization we used the \texttt{YALL-1} toolbox and set the tolerance to $10^{-4}$. For the least-squares step we use the Conjugate Gradient Least Squares instead of the well-known ``backslash'' operator in \texttt{MATLAB} since this is a well conditioned problem. For this we set the tolerance as $10^{-10}$ and the number of iterations as $10$. We have not done any code optimization such as use of \texttt{MEX} files for various sub-routines to speed up our algorithm. % \cite{yall1}

\subsubsection{Data Generation}
For the phase transition plot, for each pair of $\{b_0, r\}$ we used the Bernoulli model for sparse support generation, the low rank matrix is generated exactly as done in the previous experiments with the exception that again to provide an equal footing, we increased the ``subspace change'' by setting $\gamma_1$ and $\gamma_2$ to $10$ times the value that was used in the previous experiment. For the first $t_\train$ frames we used $b_0 = 0.02$. We provide the phase transition plots for both algorithm in Fig. \ref{fig:Comparison}. Here, white represents success while black represents failure. As can be seen, NORST is able to tolerate a much larger fraction of outlier-per-row as compared to AltProj.

\subsubsection{Real Data descriptions}
{\em Meeting Room (MR) dataset}: The meeting room sequence is set of $1964$ images of resolution $64 \times 80$. The first $1755$ frames consists of outlier-free data. Henceforth, we consider only the last $1209$ frames. For NORST, we used $t_\train=400$. In the first $400$ frames, a person wearing a black shirt walks in, writes something on the board and goes back. In the subsequent frames, the person walks in with a white shirt. This is a challenging video sequence because the color of the person and the color of the curtain are hard to distinguish. NORST is able to perform the separation at around $43$ frames per second. We present the results in Fig. \ref{fig:mr_full}

{\em Lobby (LB) dataset}: This dataset contains $1555$ images of resolution $128 \times 160$. The first $341$ frames are outlier free. Here we use the first $400$ ``noisy'' frames as training data. The Alt Proj algorithm is used to obtain an initial estimate with rank, $r = 40$. The parameters used in all algorithms are exactly the same as above. NORST achieves a ``test'' processing rate of $16$ frames-per-second. 

%--------------------------------------------
