# Supplementary material for: Fast Robust Subspace Tracking via PCA in Sparse Data-Dependent Noise
Source: arXiv:2006.08030 source file (2020-12-04)
Supplement: Supplementary file 3 [file norst_it_appendix.tex]

%\section*{Supplementary Material}
%%\appendices
%In this supplement we provide the proofs of all the results stated in the main paper. The supplement is organized as follows. We first prove preliminary results that are fundamental to our analysis in  Appendix \ref{app:concm}. We then present the proof of Theorem \ref{thm1} in Appendix \ref{sec:proof}. In Appendix \ref{sec:proof_reprocs-pca-mc} we prove the results for the extensions.







\begin{comment}

{\cb
Now, we set $\lthres = 0.59 \lambda^- \SE_j (\SE_j - 8 \zz \sqrt{f})$ (it is equal to the lower bound in item (a)). Notice that if the subspace change is such that $\SE_j < 8 \zz \sqrt{f}$, the subspace change is not detected. However, as long as $SE_j \geq 10 \zz \sqrt{f}$, we have
\begin{align*}
0.59 \lambda^- \SE_j (\SE_j - 8 \zz \sqrt{f}) \geq 0.59 \lambda^- \cdot 20 \zz^2 f > 1.37 \zz^2 f
\end{align*}
and thus this change is detected.
}

{\cred old, keeping for now, to delete later if all works out
We now obtain a lower bound on the second term in the rhs above.
\begin{align}
\lambda_{\max}(\bm{R}_j \bm{R}_j{}') &= \lambda_{\max}(\P_j{}'(\I - \Phat_{j-1}\Phat_{j-1}{}')\P_j)) = \lambda_{\max}(\P_j{}'(\I - \P_{j-1}\P_{j-1}{}' + \P_{j-1}\P_{j-1}{}' - \Phat_{j-1}\Phat_{j-1}{}')\P_j)) \nonumber \\
&\geq \lambda_{\max}(\P_j{}' (\I - \P_{j-1}\P_{j-1}{}')\P_j) + \lambda_{\min}(\P_j{}'(\P_{j-1}\P_{j-1}{}' - \Phat_{j-1}\Phat_{j-1}{}')\P_j) \nonumber \\
&= \sigma_{\max}^2((\I - \P_{j-1}\P_{j-1}{}')\P_j) + \lambda_{\min}(\P_j{}'(\P_{j-1}\P_{j-1}{}' - \Phat_{j-1}\Phat_{j-1}{}')\P_j) \nonumber \\
&\geq \SE^2(\P_{j-1}, \P_j) -\norm{\P_j{}'(\P_{j-1}\P_{j-1}{}' - \Phat_{j-1}\Phat_{j-1}{}')\P_j} \nonumber \\
&\overset{(a)}{\geq} \SE^2(\P_{j-1}, \P_j) -\norm{\P_{j-1}\P_{j-1}{}' - \Phat_{j-1}\Phat_{j-1}{}'} \geq \SE^2(\P_{j-1}, \P_j) - 2\zz
\end{align}
where we have used \cite[Lemma 2.10]{rrpcp_perf}. %$(a)$ follows from \cite{rrpcp_perf}.
Thus, combining \eqref{eq:lmaxzero}, \eqref{eq:lmaxone}, \eqref{eq:nine}, and using $\epsilon_0 = 0.01$,  $\epsilon_1 = \epsilon_2 = 0.01$, with probability at least $1 - 10n^{-10}$,
\begin{align*}
\lambda_{\max} \left( \frac{1}{\alpha} \sum_{t \in \J^{\alpha}} \bphi \lhatt \lhatt{}' \bphi \right) \geq &\ 0.99 \lambda^-(\SE^2(\P_{j-1}, \P_j) - 2\zz) - \lambda^+[\sqrt{b_0} q_0 (1.01 q_0 + 2.02 (\zz + \SE(\P_{j-1}, \P_j)))] \\
&\overset{(a)}{\geq} \lambda^- \left[0.91 \SE^2(\P_{j-1}, \P_j) - 2.7 \sqrt{b_0} f (\zz + \SE(\P_{j-1}, \P_j)^2\right]   \\
&\overset{(b)}{\geq} \lambda^-\left[ 0.91 \SE^2(\P_{j-1}, \P_j) - 0.54(\zz^2 + \SE^2(\P_{j-1}, \P_j)\right]  \\
&\geq \lambda^-\SE^2(\P_{j-1}, \P_j)(0.91 - 0.54 \cdot 1.16) \geq 0.28 \lambda^- \SE^2(\P_{j-1}, \P_j)
\end{align*}
where $(a)$ uses $q_0 = 1.2(\zz + \SE(\P_{j-1}, \P_j))$ and $\zz \leq 0.03 \SE^2(\P_{j-1}, \P_j)/f^2 < 0.4\SE^2(\P_{j-1}, \P_j)$, $(b)$ uses $\sqrt{b_0} f = 0.1$ and $(a+b)^2 \leq 2(a^2 + b^2)$. and the last inequality again uses $\zz \leq 0.03 \SE^2(\P_{j-1}, \P_j)/f^2$.
}

\end{comment}


%\subsection{Main idea of the proof} \label{only_outline}
%It is not hard to see that the ``noise'' $\b_t:=\bm\Psi (\lt+ \vt)$ seen by the projected CS step is proportional the error between the subspace estimate from $(t-1)$ and the current subspace. %Using the RIP arguments given above, and the outlier magnitudes' lower bound assumption, one can ensure that the CS step output is accurate enough and the outlier support $\T_t$ is correctly recovered. With this,
%Moreover, incoherence (denseness) of the $\P_{(t)}$'s and slow subspace change together imply that $\bpsi$ satisfies the restricted isometry property (RIP) \cite{rrpcp_perf}.
%Using this, a result for noisy $l_1$ minimization \cite{candes_rip}, and the lower bound assumption on outlier magnitudes, one can ensure that the CS step output is accurate enough and the outlier support $\T_t$ is correctly recovered. With this, we have that $\lhat_t = \lt + \vt - \et$ where $\et:=\x_t -\xhat_t$ satisfies
%$
%\et= \I_{\T_t} (\bm\Psi_{\T_t}{}'\bm\Psi_{\T_t})^{-1} \I_{\T_t}{}' \bm\Psi' \lt
%$
%and $\|\et\| \le C \|\b_t\|$. %\le C \SE(\Phat_{(t-1)},\P_{(t)}) \|\at\|$.
%%
%Consider subspace update. Every time the subspace changes, one can show that the change can be detected within a short delay. After that, the $K$ SVD steps help get progressively improved estimates of the changed subspace. To understand this, observe that, after a subspace change, but before the first update step, $\b_t$ is the largest and hence, $\et$, is also the largest for this interval. However, because of good initialization or because of slow subspace change and previous subspace correctly recovered (to error $\zz$), neither is too large. Both are proportional to $(\zz + \dif)$, or to the initialization error. %Recall that $\dif$ quantifies the amount of subspace change. For simplicity suppose that $\SE(\Phat_0,\P_0) = \dif$.
%Using the idea below, we can show that we get a ``good'' first estimate of the changed subspace.
%
%The input to the PCA step is $\lhat_t$ and the noise seen by it is $\et$. Notice that $\et$ depends on the true data $\lt$. Hence this is a setting of PCA in data-dependent noise \cite{corpca_nips,pca_dd}.
%From \cite{pca_dd}, it is known that the subspace recovery error of the PCA step is proportional to the ratio between the time averaged noise power plus time-averaged signal-noise correlation, $(\|\sum_t \E[\et \et{}']\| + \|\sum_t \E[\lt \et{}'\|)/\alpha$, and the minimum signal space eigenvalue, $\lambda^-$.
%The instantaneous value of noise power is $(\dif+\zz)^2$ times $\lambda^+$ while that of signal-noise correlation is of order $(\dif+\zz)$ times $\lambda^+$. However, using the fact that $\et$ is sparse with support $\T_t$ that changes enough over time so that $\outfracrow(\alpha)$ is bounded, one can argue (using Cauchy-Schwartz) that their time averaged values are $\sqrt{\outfracrow(\alpha)}$ times smaller. As a result, after the first subspace update, the subspace recovery error is at most $4 \sqrt{\outfracrow(\alpha)} (\lambda^+/\lambda^-)$ times $(\dif+\zz)$. Since $\outfracrow(\alpha) (\lambda^+/\lambda^-)^2$ is bounded by a constant $c_2 < 1$, this means that, after the first subspace update, the subspace error is at most $\sqrt{c_2}$ times $(\dif+\zz)$.
%
%This, in turn, implies that $\|\b_t\|$, and hence $\|\et\|$, is also $\sqrt{c_2}$ times smaller in the second subspace update interval compared to the first. This, along with repeating the above argument, helps show that the second estimate of the changed subspace is $\sqrt{c_2}$ times better than the first and hence its error is $(\sqrt{c_2})^2$ times $(\dif+\zz)$. Repeating the argument $K$ times, the $K$-th estimate has error $(\sqrt{c_2})^K$ times $(\dif+\zz)$. Since $K = C \log(1/\zz)$, this is an $\zz$ accurate estimate of the changed subspace.
%
%%A careful application of the \cite{pca_dd} result and the following fact is the main reason why we are able to remove the moving object model assumption on the outlier support
%%The reason why we are able to remove the moving object model assumption on the outlier support is as follows
%A careful application of the result of \cite{pca_dd} is the reason why we are able to remove the moving object model assumption on the outlier support needed by the earlier guarantees for original-ReProCS \cite{rrpcp_isit15,rrpcp_aistats}. Applied to our problem, this result requires $\|\sum_{t \in \J(\alpha)} \itt \itt{}' /\alpha\|$ to be bounded by a constant less than one. It is not hard to see that $\max_{\J^\alpha \in [1,\tmax]} \|\sum_{t \in \J^\alpha} \itt \itt{}'/\alpha\| = \outfracrow^{\alpha}$. To understand this simply, the matrix $\sum_{t \in \J^\alpha} \itt \itt{}'$ is diagonal, and the $i$-th diagonal entry counts the number of time the index $i$ appears in the support set $\T_t$ in the interval $\J^{\alpha}$ which is precisely the definition of $\outfracrow^{\alpha} \cdot \alpha$. This is also why a constant bound on $\outfracrow^{\alpha}$ suffices for our setting. On the other hand the guarantees of \cite{rrpcp_isit15,rrpcp_aistats} required that, for any sequence of positive semi-definite (p.s.d.) matrices, $\A_t$, $\|\sum_{t \in \J^\alpha} \itt \A_t \itt{}' /\alpha\|$,  be bounded by a constant less than one. This is a much more stringent requirement; one way to satisfy it is using the moving object model on outlier supports assumed there.
